# Supplementary material for: Time Weaver: A Conditional Time Series Generation Model
Source: arXiv:2403.02682 source file (2026-12-03)
Supplement: Supplementary file 1 [file main_table_duplicate.tex]

 % Please add the following required packages to your document preamble:
% \usepackage{graphicx}
\begin{table*}
\centering
% \resizebox{0.8\textwidth}{!}{%
\begin{sc}
\begin{tabular}{lcccccccc}
\hline
\multirow{2}{*}{Approach} & \multicolumn{2}{c}{Air Quality} & \multicolumn{2}{c}{ECG} & \multicolumn{2}{c}{Traffic} & \multicolumn{2}{c}{Electricity} \\ 
                          & J-FTSD       & TSTR     & J-FTSD    & TSTR   & J-FTSD      & TSTR     & J-FTSD         & TSTR        \\ \hline
WaveGAN \\
\cite{donahue2019wavegan}  & 10 & 0.713 & X & X & 28 & 0.64 & X & X \\ \hline
Pulse2Pulse \\
\cite{thambawita2021pulse2pulse}  & 35 & 0.6 & 0.2457 & X & 27 & 0.57 & 0.6416 & X \\ \hline
\timeweaver-CSDI   & \textbf{6} & \textbf{0.785} & 0.1396 & X & 1.01 & \textbf{0.896} & \textbf{0.0029} & \textbf{0.8422}  \\ \hline
\timeweaver-SSSD    & 8 & 0.712 & \textbf{0.0688} & X & \textbf{0.34} & 0.891 & 0.0144 & 0.83  \\ \hline
\end{tabular}
\end{sc}
% }
\caption{\small{\textbf{Diffusion-based approaches outperform GAN-based approaches on J-FTSD metric and Train on Synthetic Test on Real (TSTR)}. The table shows the performance of all the models (rows) on specified datasets (columns). Specifically, we compare the models on J-FTSD and TSTR metrics. It can be observed that both \timeweaver \space variants consistently outperform GAN models in both metrics. Another key insight is the observed correlation between J-FTSD and TSTR trends. Our experimental findings indicate that lower FTSD scores correspond to higher Area Under the Curve (AUC) scores when tested on the original test dataset.}}

\label{tab:quant_comp_1}
\end{table*}

\begin{table*}
\centering
% \resizebox{0.8\textwidth}{!}{%
\begin{sc}
\begin{tabular}{lcccccccc}
\hline
\multirow{2}{*}{Approach} & \multicolumn{2}{c}{Air Quality} & \multicolumn{2}{c}{ECG} & \multicolumn{2}{c}{Traffic} & \multicolumn{2}{c}{Electricity} \\ 
                          & J-FTSD       & TSTR     & J-FTSD    & TSTR   & J-FTSD      & TSTR     & J-FTSD         & TSTR        \\ \hline
WaveGAN \\
\cite{donahue2019wavegan}  & 10 & 0.862 & X & X & X & X & X & X \\ \hline
Pulse2Pulse \\
\cite{thambawita2021pulse2pulse}  & 35 & 0.72 & 0.2457 & X & 0.9547 & X & 0.6416 & X \\ \hline
\timeweaver-CSDI   & \textbf{6} & \textbf{0.874} & 0.1396 & X & 0.0237 & X & \textbf{0.0029} & \textbf{0.8422}  \\ \hline
\timeweaver-SSSD    & 8 & 0.862 & \textbf{0.0688} & X & \textbf{0.0112} & X & 0.0144 & 0.83  \\ \hline
\end{tabular}
\end{sc}
% }
\caption{\small{\textbf{Diffusion-based approaches outperform GAN-based approaches on J-FTSD metric and Train on Synthetic Test on Real (TSTR)}. The table shows the performance of all the models (rows) on specified datasets (columns). Specifically, we compare the models on J-FTSD and TSTR metrics. It can be observed that both \timeweaver \space variants consistently outperform GAN models in both metrics. Another key insight is the observed correlation between J-FTSD and TSTR trends. Our experimental findings indicate that lower FTSD scores correspond to higher Area Under the Curve (AUC) scores when tested on the original test dataset.}}

\label{tab:quant_comp_2}
\end{table*}
