# Supplementary material for: Time Weaver: A Conditional Time Series Generation Model
Source: arXiv:2403.02682 source file (2026-12-03)
Supplement: Supplementary file 2 [file algorithm.tex]

\begin{algorithm}
	\caption{One epoch in the feature extractors' ($\metricembedderts$ and $\metricembeddercondn$) training}
    \begin{algorithmic}[1]
        \STATE {\bfseries Input:} Time Series feature extractor $\metricembedderts$, Metadata feature extractor $\metricembeddercondn$, Dataset $\dataset$, Batch Size $\batchsize$, Number of patches $\patchsize$, Patch Length $\patchlength$
        
        \FORALL{sampled batch $\{\timeseries_i, \condition_i\}_{i=1}^{\batchsize} \subset \dataset$} 
        \STATE $X_{\textnormal{patch}},C_{\textnormal{patch}}  = \emptyset, \emptyset$
        \FORALL{$i \in \{1,\ldots, \batchsize$\}}
        \STATE Randomly sample $\patchsize$ patches of length $\patchlength$ from $\timeseries_i$ and $\condition_i$ and append them to $X_{\textnormal{patch}}$ and $C_{\textnormal{patch}}$ respectively.  \alglinelabel{ln:sample_patch}
        \ENDFOR
        \STATE Obtain the time series and the metadata embeddings of the sampled patches $Z_{\textnormal{time}} = \{ \metricembedderts(\timeseries) : \forall \timeseries \in X_{\textnormal{patch}}\}$ , $Z_{\textnormal{meta}} = \{\metricembeddercondn(\condition) : \forall \condition \in C_{\textnormal{patch}}\}$ \alglinelabel{ln:process_patch}
        \STATE Let $N_{\textnormal{samples}} = \batchsize \times \patchsize$
        \FORALL{$i \in \{1,\ldots, N_{\textnormal{samples}}\}$}
        \FORALL{$j \in \{1,\ldots, N_{\textnormal{samples}}\}$}
        \STATE $s_{i,j} = Z_{\textnormal{time}}[i]^\top Z_{\textnormal{meta}}[j]$ \alglinelabel{ln:dotproduct}     
        \ENDFOR
        \ENDFOR
        \STATE \textbf{define} $l(i,j)$ \textbf{as} $l(i,j) = -\textnormal{log}\frac{\textnormal{exp}(s_{i,j})}{\sum_{k=1}^{N_{\textnormal{samples}}} \textnormal{exp}(s_{i,k})}$ \alglinelabel{ln:cross_entropy} 
        \STATE $\mathcal{L}_{\textnormal{CE}} = \frac{1}{N_{\textnormal{samples}}} \sum_{i , j } l(i,j) + \frac{1}{N_{\textnormal{samples}}} \sum_{j , i } l(j,i)$ \alglinelabel{ln:CE_loss}
        \STATE Update $\metricembedderts$ and $\metricembeddercondn$ to minimize $\mathcal{L}_{\textnormal{CE}}$
        \ENDFOR
    \end{algorithmic}  
\label{alg:metric_training}
\end{algorithm}
