# Supplementary material for: Time Weaver: A Conditional Time Series Generation Model
Source: arXiv:2403.02682 source file (2026-12-03)
Supplement: Supplementary file 3 [file experiment_details.tex]

\section{Experiment Details}
\label{appendix:experiment_details}
